# Supplementary material for: Speeding Up Multi-Objective Hyperparameter Optimization by Task Similarity-Based Meta-Learning for the Tree-Structured Parzen Estimator
Source: arXiv:2212.06751 source file (2023-05-31)
Supplement: Supplementary file 1 [file hp-importance.tex]

\subsection{Proof of Proposition \ref{main:methods:proposition:hp-importance}}
\label{appendix:proofs:subsection:proof-of-hp-importance}
We first introduce the following marginal
mean of the binary function $b(\xv | \Xg)$ for the proof:
\begin{definition}[Marginal mean]
  \begin{equation}
    \begin{aligned}
      q(x_i | \Xg) \coloneqq \int_{\xv \in \X} b(\xv | \Xg) \frac{\mu(d\xv_{-i})}{\mu(\X_{-i})}
    \end{aligned}
  \end{equation}
  where $\xv_{-i} \in \mathbb{R}^{D - 1}$ is $\xv$
without the $i$-th dimension.
\end{definition}
We also note that the following holds by definition of the binary function:
\begin{equation}
  \begin{aligned}
    \gamma = \int_{\xv \in \X} b(\xv | \Xg) \frac{\mu(d\xv)}{\mu(\X)}.
  \end{aligned}
  \label{appendix:proofs:eq:binary-expectation-is-gamma}
\end{equation}
Then we first prove the following lemma:
\begin{lemma}
  The following holds:
  \begin{equation}
    \begin{aligned}
      \int_{x_i \in \X_i} q(x_i | \Xg)\frac{\mu(dx_i)}{\mu(\X_i)} = \gamma
    \end{aligned}
  \end{equation}
  \label{appendix:proofs:lemma:integral-of-marginalized-dist}
\end{lemma}
\begin{proof}
  By definition, the following equality holds:
  \begin{equation}
    \begin{aligned}
      \int_{x_i \in \X_i} q(x_i | \Xg)\frac{\mu(dx_i)}{\mu(\X_i)} =
      \int_{x_i \in \X_i} \int_{\xv_{-i} \in \X_{-i}} b(\xv | \Xg)
      \frac{\mu(dx_{-i})}{\mu(\X_{-i})}
      \frac{\mu(dx_i)}{\mu(\X_i)}.
    \end{aligned}
  \end{equation}
  Since the Lebesgue measure is a product measure
  and $b(\xv | \Xg) \geq 0$,
  the Fubini's theorem holds, and thus we obtain the following:
  \begin{equation}
    \begin{aligned}
      \mathrm{LHS} = \int_{\xv \in \X} b(\xv | \Xg) \frac{\mu(d\xv)}{\mu(\X)} 
      = \gamma~(\because \mathrm{Eq.~}(\ref{appendix:proofs:eq:binary-expectation-is-gamma})).
    \end{aligned}
  \end{equation}
  This completes the proof.
\end{proof}
Using this lemma, we prove Proposition~\ref{main:methods:proposition:hp-importance}.
\begin{proof}
  Since $b(\xv | \Xg)$ is a special version, such that $k(\xv, \xv^\prime) = \delta(\xv, \xv^\prime)$,
  of the $\gamma$-set PDF,
  the marginalization of $b(\xv | \Xg)$ is viewed as the marginalization
  of $p(\xv | \Xg)$ with a different scale.
  From Lemma~\ref{appendix:proofs:lemma:integral-of-marginalized-dist},
  the scale to equalize this marginalization is $\gamma\mu(\X_i)$,
  and thus the marginal $\gamma$-set PDF
  is computed as $p(x_i | \Xg) = q(x_i | \Xg) / (\gamma \mu(\X_i))$.
  Therefore, we obtain the following marginal variance:
  \begin{equation}
    \begin{aligned}
      \mathbb{V}_i &\coloneqq \mathbb{E}[(q(x_i | \Xg) - \gamma)^2] \\
      &= \mathbb{E}[(\gamma \mu(\X_i)p(x_i | \Xg) - \gamma)^2]\\
      &= (\gamma \mu(\X_i) )^2 \mathbb{E}\Biggl[
        \Biggl(p(x_i | \Xg) - \frac{1}{\mu(\X_i)}
        \Biggr)^2
        \Biggr]
    \end{aligned}
  \end{equation}
  and this completes the proof.
\end{proof}
As seen in the equation above,
the marginal variance is measured
via the L2 norm between the uniform PDF and
the marginal $\gamma$-set PDF.
We can rank each dimension by $\mathbb{V}_i$.
